# Supplementary material for: Compressing RNNs for IoT devices by 15-38x using Kronecker Products
Source: arXiv:1906.02876 source file (2020-01-31)
Supplement: Supplementary file 1 [file Background.tex]

\section{Background}
\label{sec:appBackground}

\begin{figure}
  \begin{center}
  \includegraphics[width=\columnwidth]{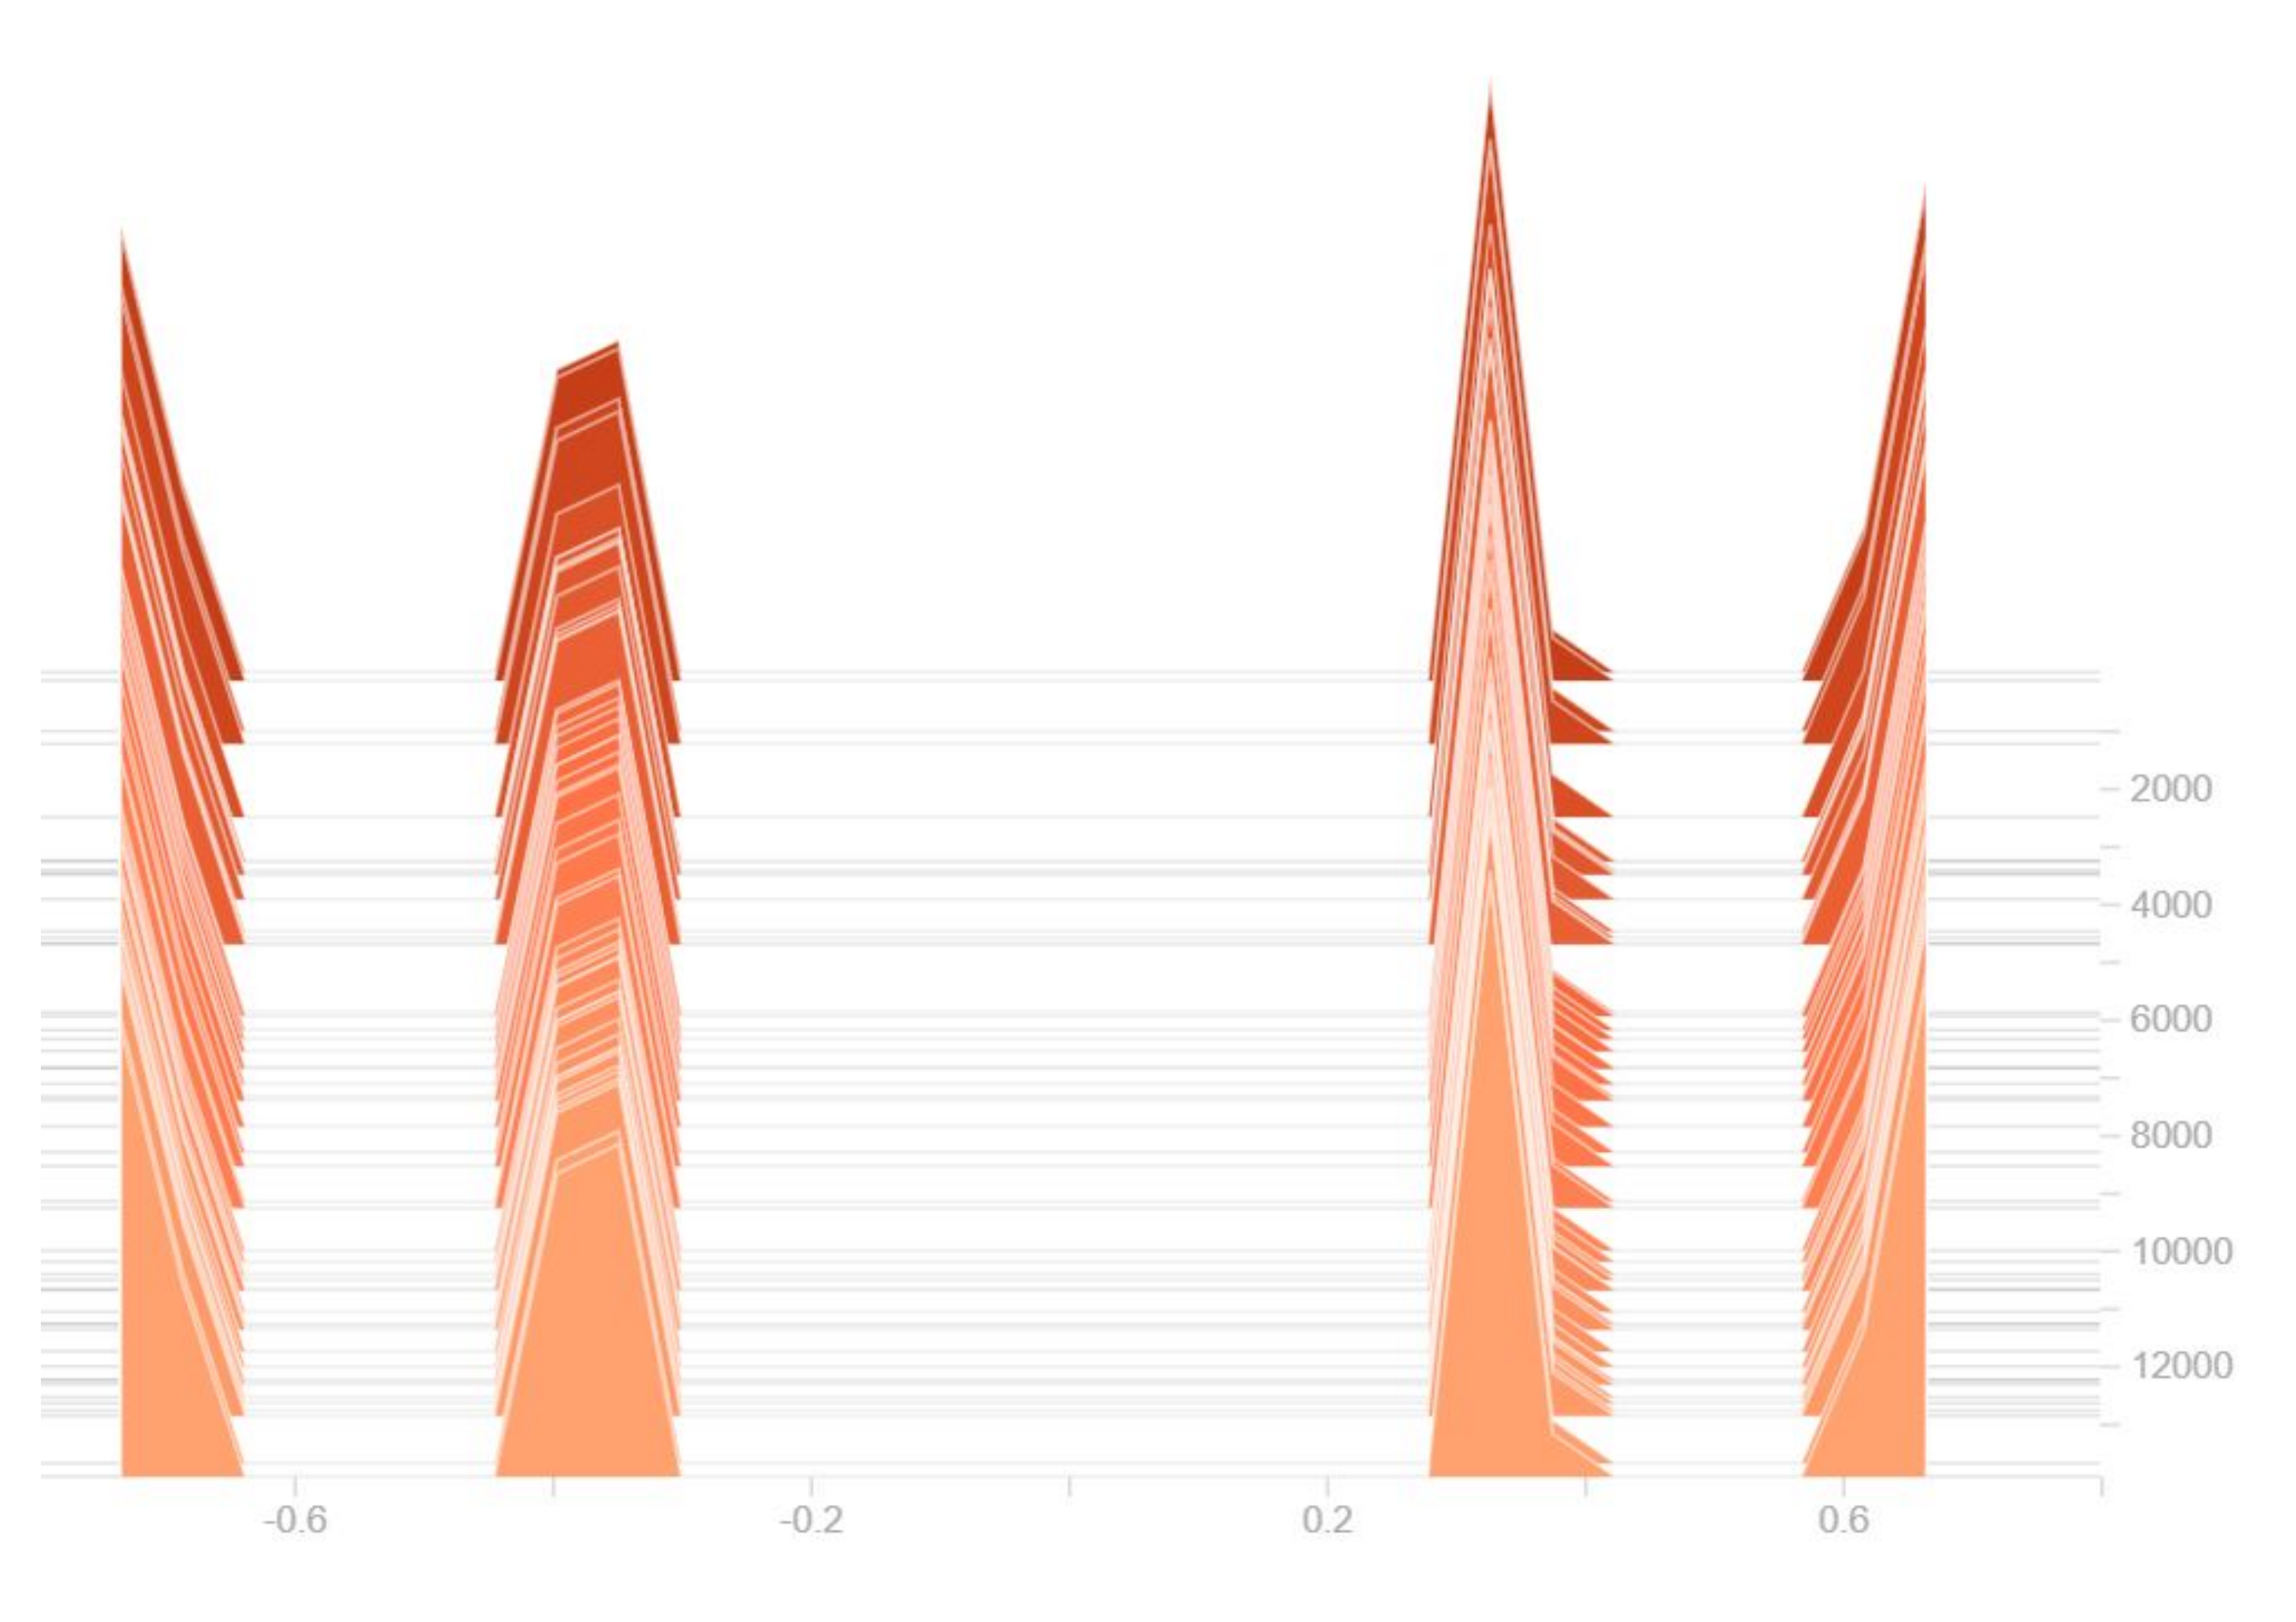}
  \caption{The values of a 2x2 matrix across multiple epochs}
  \label{fig:2x2kron}
  \end{center}
\end{figure}

We tried using the framework provided by \cite{kron1} to compress the GRU matrix in the small GRU baseline in \cite{zhang2017} by a factor of 2. We used a GRU with hidden vector size of 256 and replaced the hidden-hidden matrix with Kronecker product of 8, 2x2 matrices as described in \cite{kron1}. The resultant network lost 3\% accuracy. On inspecting the 2x2 matrices, we found that the matrices hardly changed after initialization. Figure \ref{fig:2x2kron} shows the values of a 2x2 matrix across multiple epochs during training. We see the values in the matrix do not change after initialization.
